# Supplementary material for: Unified Cross-modal Translation of Score Images, Symbolic Music, and Performance Audio
Source: arXiv:2505.12863 source file (2025-05-19)
Supplement: Supplementary file 1 [file refs_supple.tex]

\begin{thebibliography}{1}
\bibliographystyle{IEEEtran}
\bibitem{cocodataset}
T.-Y. Lin et al., ‘Microsoft COCO: Common Objects in Context’, in Computer Vision -- ECCV 2014, 2014, pp. 740–755.

\bibitem{esser2020taming}
P. Esser, R. Rombach, and B. Ommer, ‘Taming Transformers for High-Resolution Image Synthesis’, in Proceedings of the IEEE/CVF Conference on Computer Vision and Pattern Recognition (CVPR), 2021, pp. 12873–12883.

\bibitem{rodriguez2023ocr}
J. A. Rodriguez, D. Vazquez, I. Laradji, M. Pedersoli, and P. Rodriguez, ‘OCR-VQGAN: Taming Text-within-Image Generation’, in Proceedings of the IEEE/CVF Winter Conference on Applications of Computer Vision, 2023, pp. 3689–3698.

\end{thebibliography}
